# Supplementary material for: Droplet breakup in airflow with strong shear effect
Source: arXiv:2301.06271 source file (2023-01-16)
Supplement: Supplementary file 1 [file Supplementary_Material.pdf]

# Droplet breakup in airflow with strong shear effect: Supplementary material

Zhikun Xu, Tianyou Wang and Zhizhao Che<sup>†</sup>

State Key Laboratory of Engines, Tianjin University, Tianjin 300072, China

(19 February 2022)

## 1. Details of image processing for measuring fragment size based on fragment tracking

The purpose of the image processing is to count all the fragments passing through a specified boundary by tracking each fragment in an image sequence. This is achieved by the following steps:

Step 1: *Image acquisition*. Before the image processing, we need to tune the photography setting to obtain appropriate image sequences. The shooting area needs to satisfy that all fragments of the droplet breakup pass through this area. The maximum spatial resolution of the image in this study is  $40\text{ }\mu\text{m/pixel}$ . To improve the accuracy of fragment tracking, we need to ensure that the displacement of the fragments in two consecutive images is small and the outlines of the fragments are clear. Therefore, a high frame rate (30000 fps) and a short exposure time ( $1.5\text{ }\mu\text{s}$ ) are selected. Due to the dispersion of the fragments in a large area, a 60-mm macro lens (Nikon AF 60 mm f/2.8D) with a small aperture (F22) is used to obtain a large depth of field with low optical distortion to capture all fragments. Moreover, a high-power (800 W) light-emitting diode (LED) light diffused by ground glass is used as the background light source to ensure sufficient brightness.

Step 2: *Fragment detection in each image*. We firstly mask the raw image to a certain region for analysis. The region is set as a belt region of 100–200 pixels in width along the top, right, and bottom boundaries of the image where the fragments will pass through (see the light-orange region in Figure S1). Then the background of the image is removed by subtracting an image without any droplet and the image is enlarged twice by interpolation to get a finer image. Further, the image is binarised based on a threshold in the brightness, and holes in the fragments in the binary image are filled. After that, objects smaller than 20 pixels are removed from the binary image, as they have a large error in calculating the fragment size. Through these procedures, we can detect fragments in each image.

Step 3: *Prediction of fragment's location*. Each fragment corresponds to a track in the image sequence. The location of each fragment in the next frame is predicted by a Kalman

<sup>†</sup> Email address for correspondence: chezhizhao@tju.edu.cn

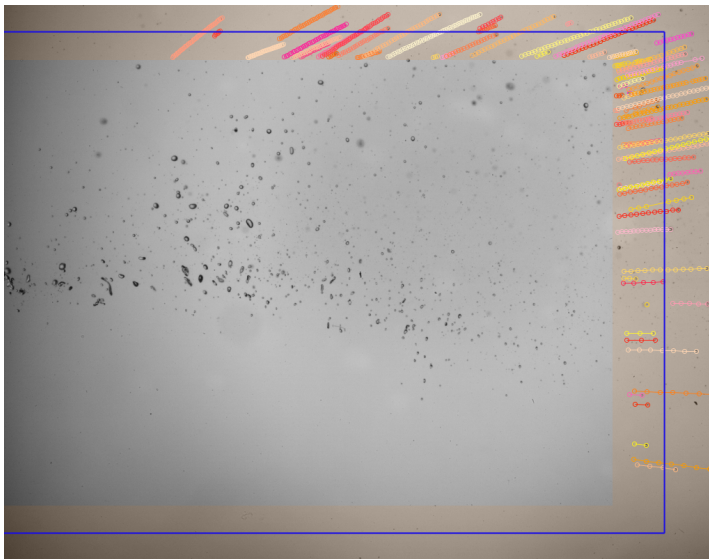

FIGURE S1. Illustration of the image processing for measuring fragment size based on fragment tracking. The light-orange region is used for fragment tracking analysis. The blue line is the specified boundary. The colored lines with circles are the tracks of fragments.

filter, in which the fragment is assumed to move at a constant acceleration. According to the predicted location, the filter determines the cost of each fragment being assigned to each track in the next frame.

Step 4: *Association of the fragments to the tracks*. Since the cost obtained in step 3 is based only on the motion of the fragment, we further calculated the weighted average of the costs based on the fragment size and the motion direction. When there is at least one weighted average cost less than a specified threshold, the fragment and the track corresponding to the minimum cost are associated. Then the track is updated using the corresponding fragment and is marked visible. However, if there is no weighted average cost less than the specified threshold, the track is not associated with any fragments and is marked invisible. Finally, the remaining fragments that are not associated with any tracks will be used to start a new track.

Step 5: *Calculation of fragment size*. By repeating Steps 2–4 for all image sequences, we can obtain the tracks of all fragments (the colored lines with circles in figure S1). The tracks which are marked visible less than 4 times are considered as a failure to continuously track the fragments. Finally, the size of fragments corresponding to the tracks passing through the specified boundary (the blue line in figure S1) is calculated from the number of pixels of the fragment in the image by using a scaling factor.

A typical tracking process of the fragments generated by droplet breakup is shown in movie 10.
